# Supplementary material for: Assurance via workflow+ modelling and conformance
Source: arXiv:1912.09912 source file (2019-12-20)
Supplement: Supplementary file 1 [file backgr-in-appendix.tex]

\section{Background: Assurance cases and GSN} 

The long history of safety assurance can roughly be divided in two periods. In the first one, the certifying authority regulated the design (D) and manufacturing process (M) so that the product had been considered safe if D and M satisfied the prescribed \req s. However, such prescriptive regulations turned out limiting technical innovations (including safety innovations if designed after the time of regulation is written; an in-depth discussion of  these and other deficiencies can be found in \cite{pppf-bloomf-10}). Another approach had been getting popular since the mid-nineties by requiring the (original equipment) manufacturer (OEM) to submit to the certifying authority a {\em safety case (SC)}: ``a documented body of evidence that provides a convincing and valid argument that a system is adequately safe for a given application in a given environment'' \zdhll{\cite{?}}{ref to ASCAD, 1998}{-3ex}. The approach turned out effective and currently dominates the assurance domain \zdhll{\cite{?,?}.}{1-2 refs are needed}{0.5ex}

\endinput
